# Supplementary material for: CRAFT: Contextual Re-Activation of Filters for face recognition Training
Source: arXiv:2312.00072 source file (2023-12-05)
Supplement: Supplementary file 1 [file classification.tex]

\begin{figure*}[ht!]
 \centering
  \begin{subfigure}[b]{0.9\linewidth}
      \begin{subfigure}[b]{0.3\linewidth}
        \centering
          \includegraphics[width=1\linewidth]{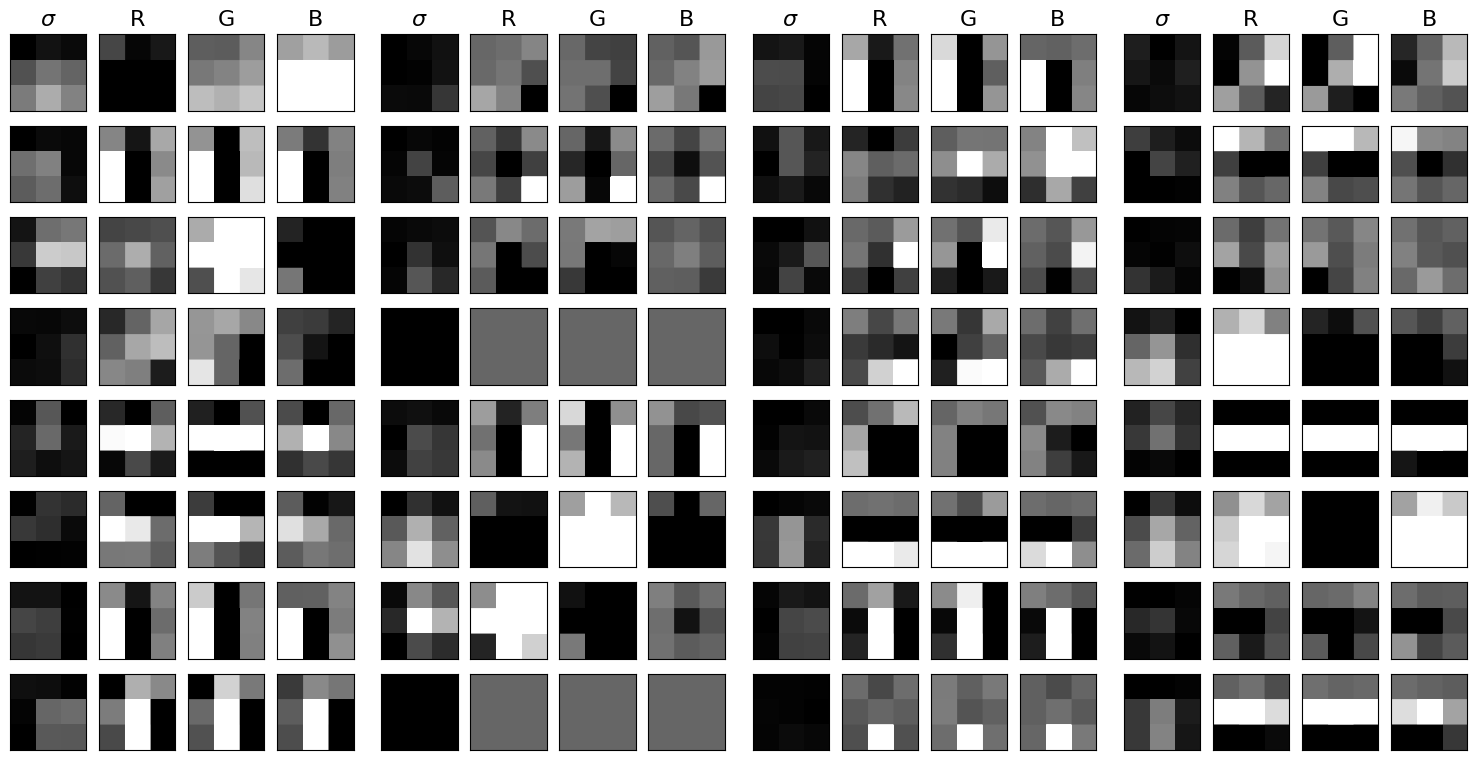}
          \caption{\scriptsize{mobilenet}}\label{arcface_meanshift}
      \end{subfigure}
      \hfill
      \begin{subfigure}[b]{0.3\linewidth}
        \centering
          \includegraphics[width=1\linewidth]{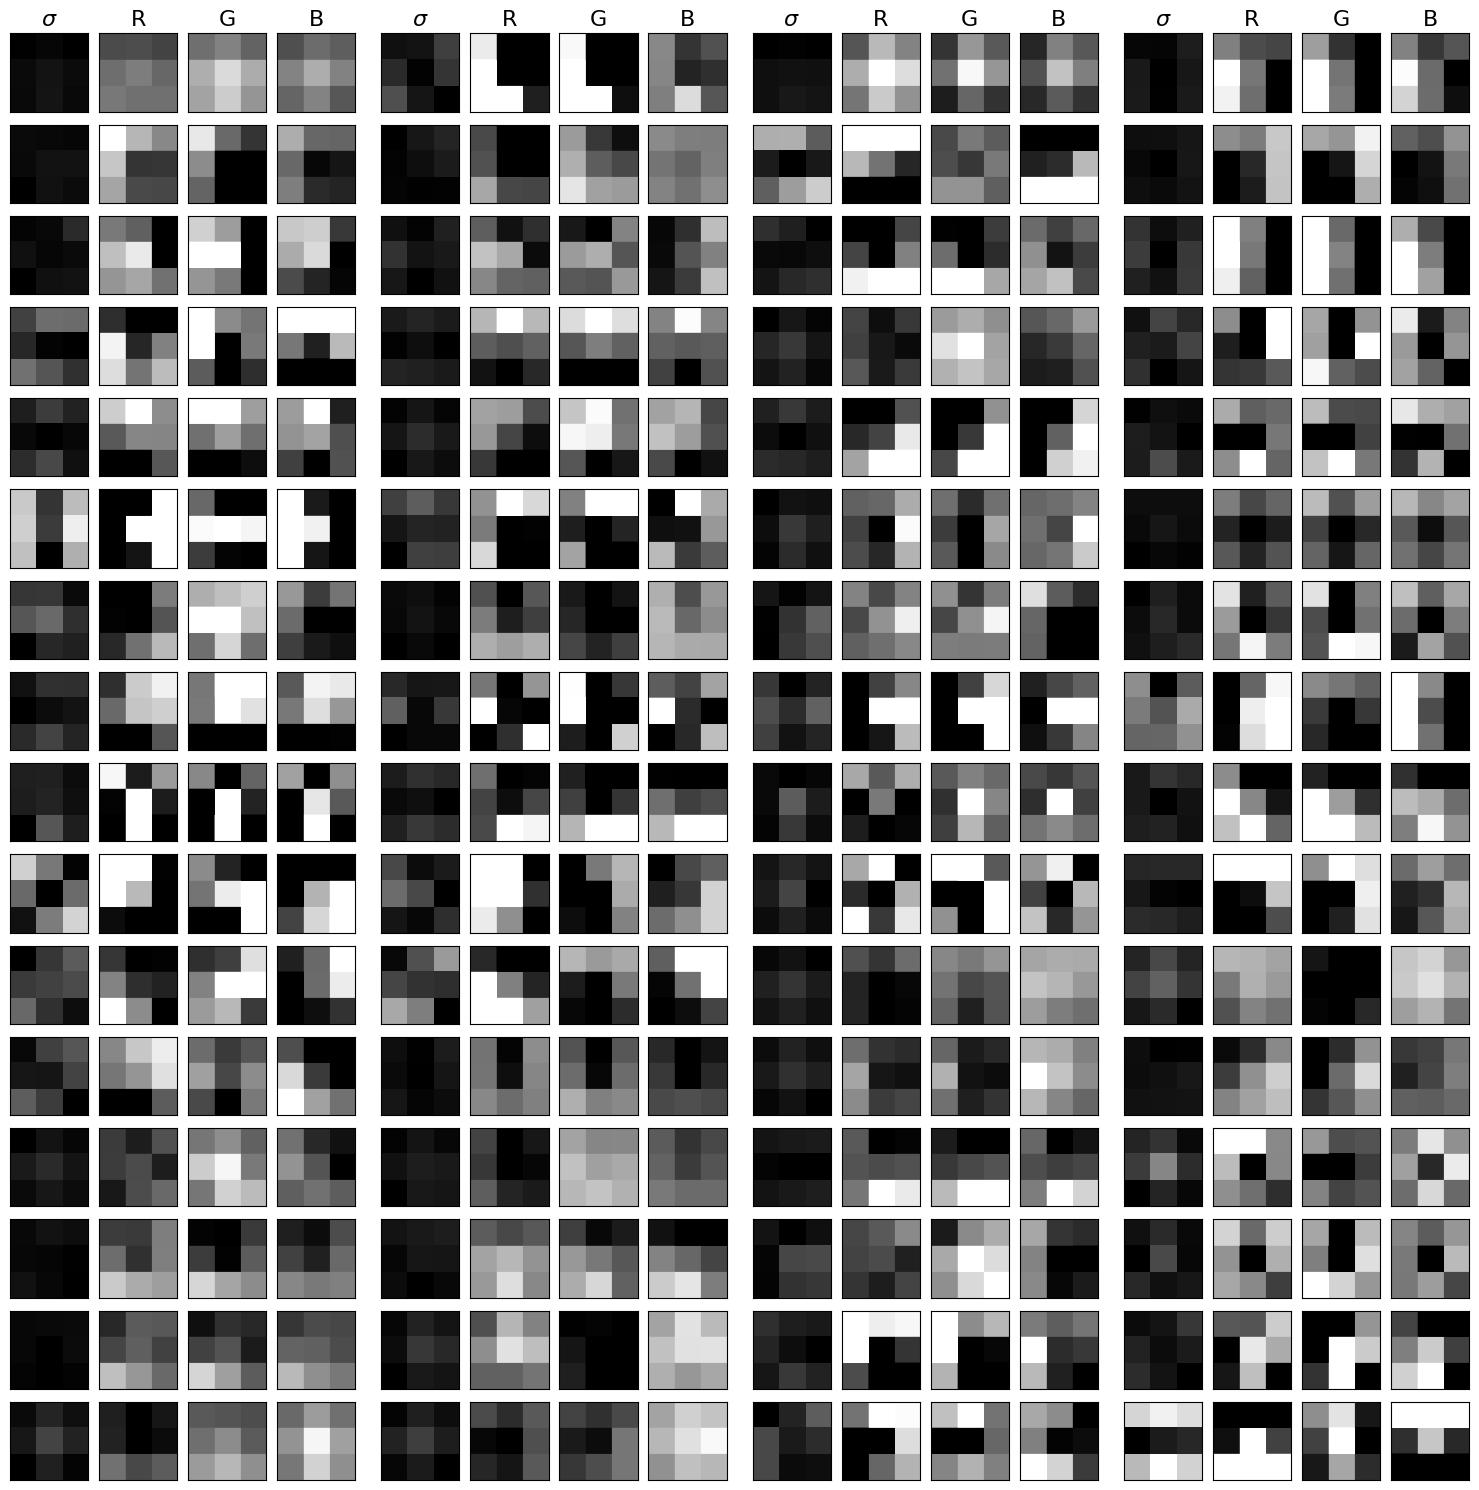}
          \caption{\scriptsize{vgg19}}\label{magface_meanshift}
      \end{subfigure}
      \hfill
      \begin{subfigure}[b]{0.3\linewidth}
        \centering
          \includegraphics[width=1\linewidth]{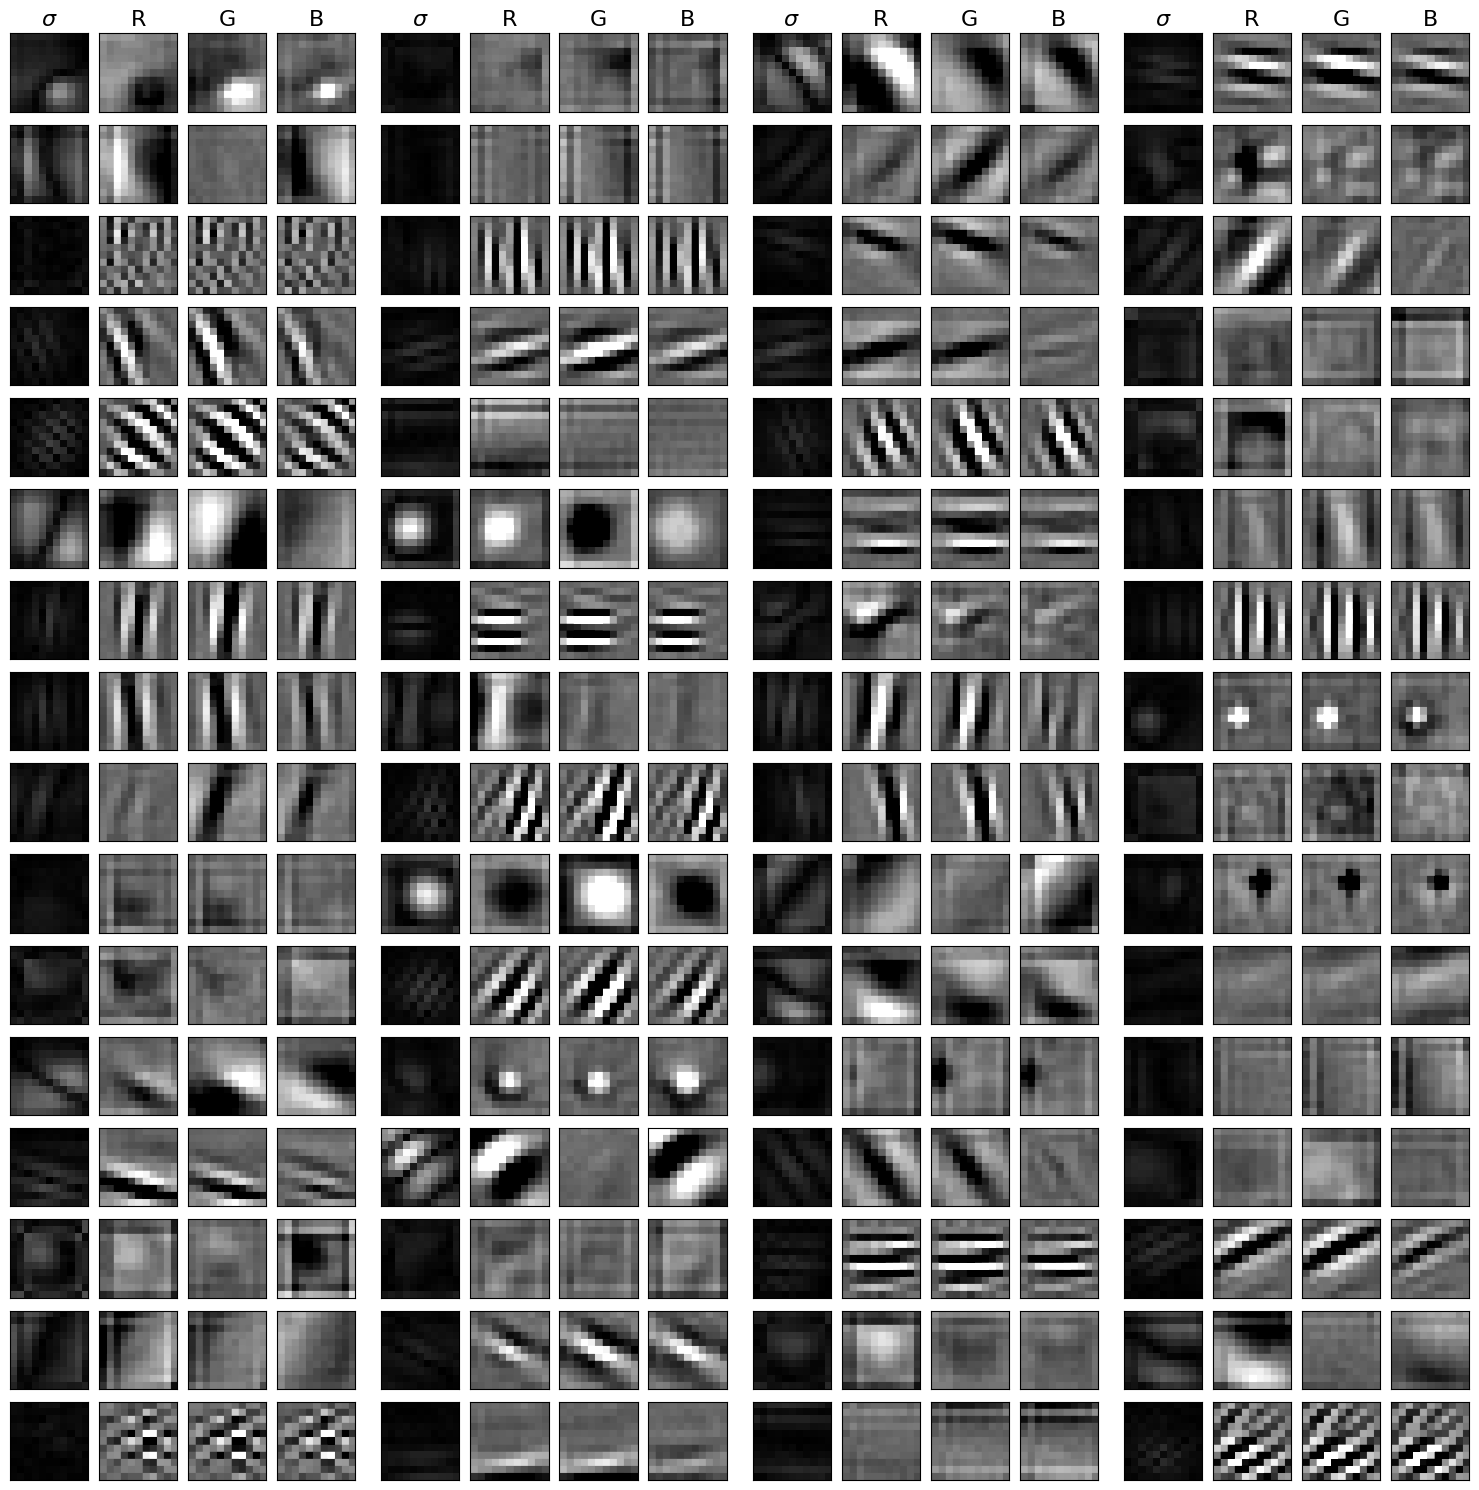}
          \caption{\scriptsize{alexnet}}\label{magface_meanshift}
      \end{subfigure}
    \end{subfigure}
    \begin{subfigure}[b]{0.9\linewidth}
      \begin{subfigure}[b]{0.3\linewidth}
        \centering
          \includegraphics[width=1\linewidth]{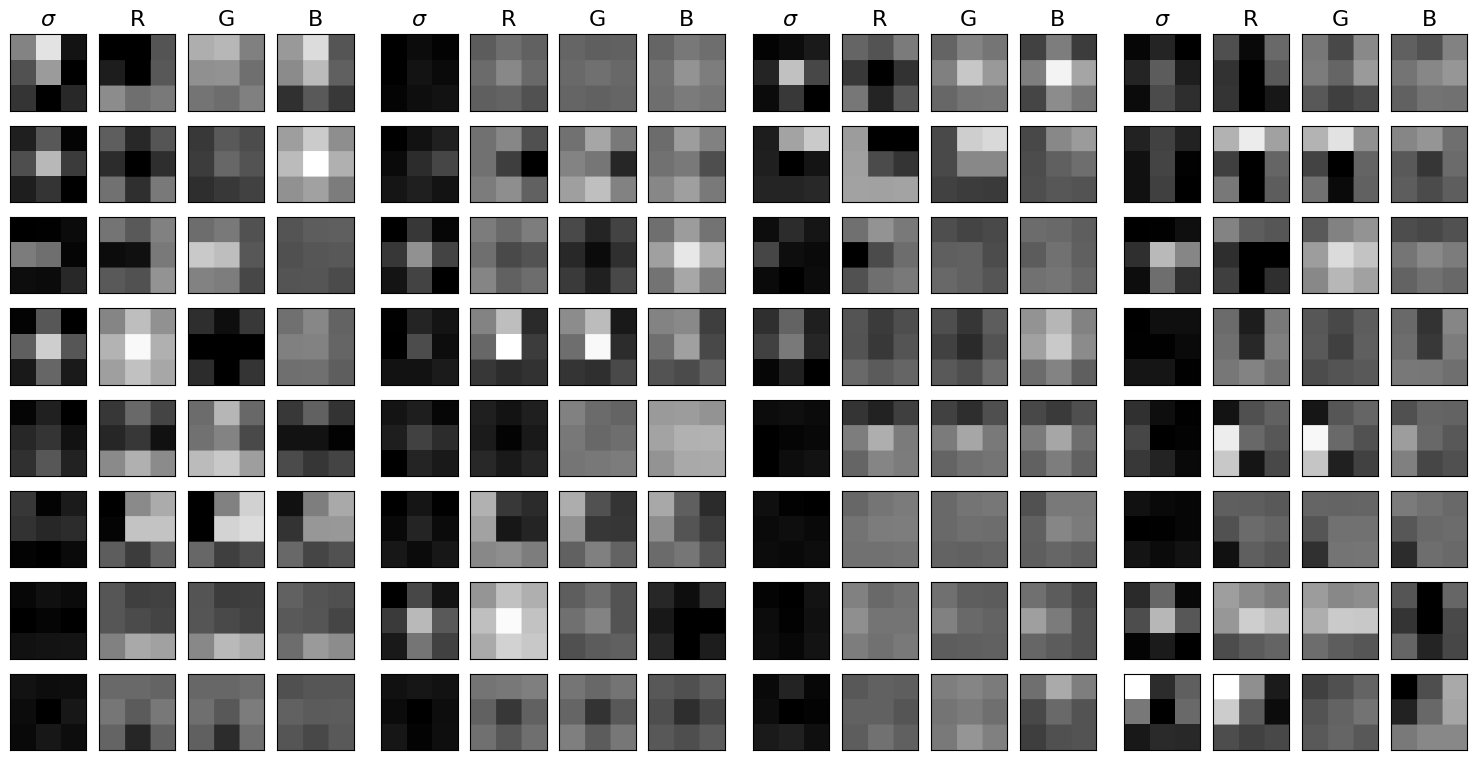}
          \caption{\scriptsize{inception\_v2}}\label{arcface_meanshift}
      \end{subfigure}
      \hfill
      \begin{subfigure}[b]{0.3\linewidth}
        \centering
          \includegraphics[width=1\linewidth]{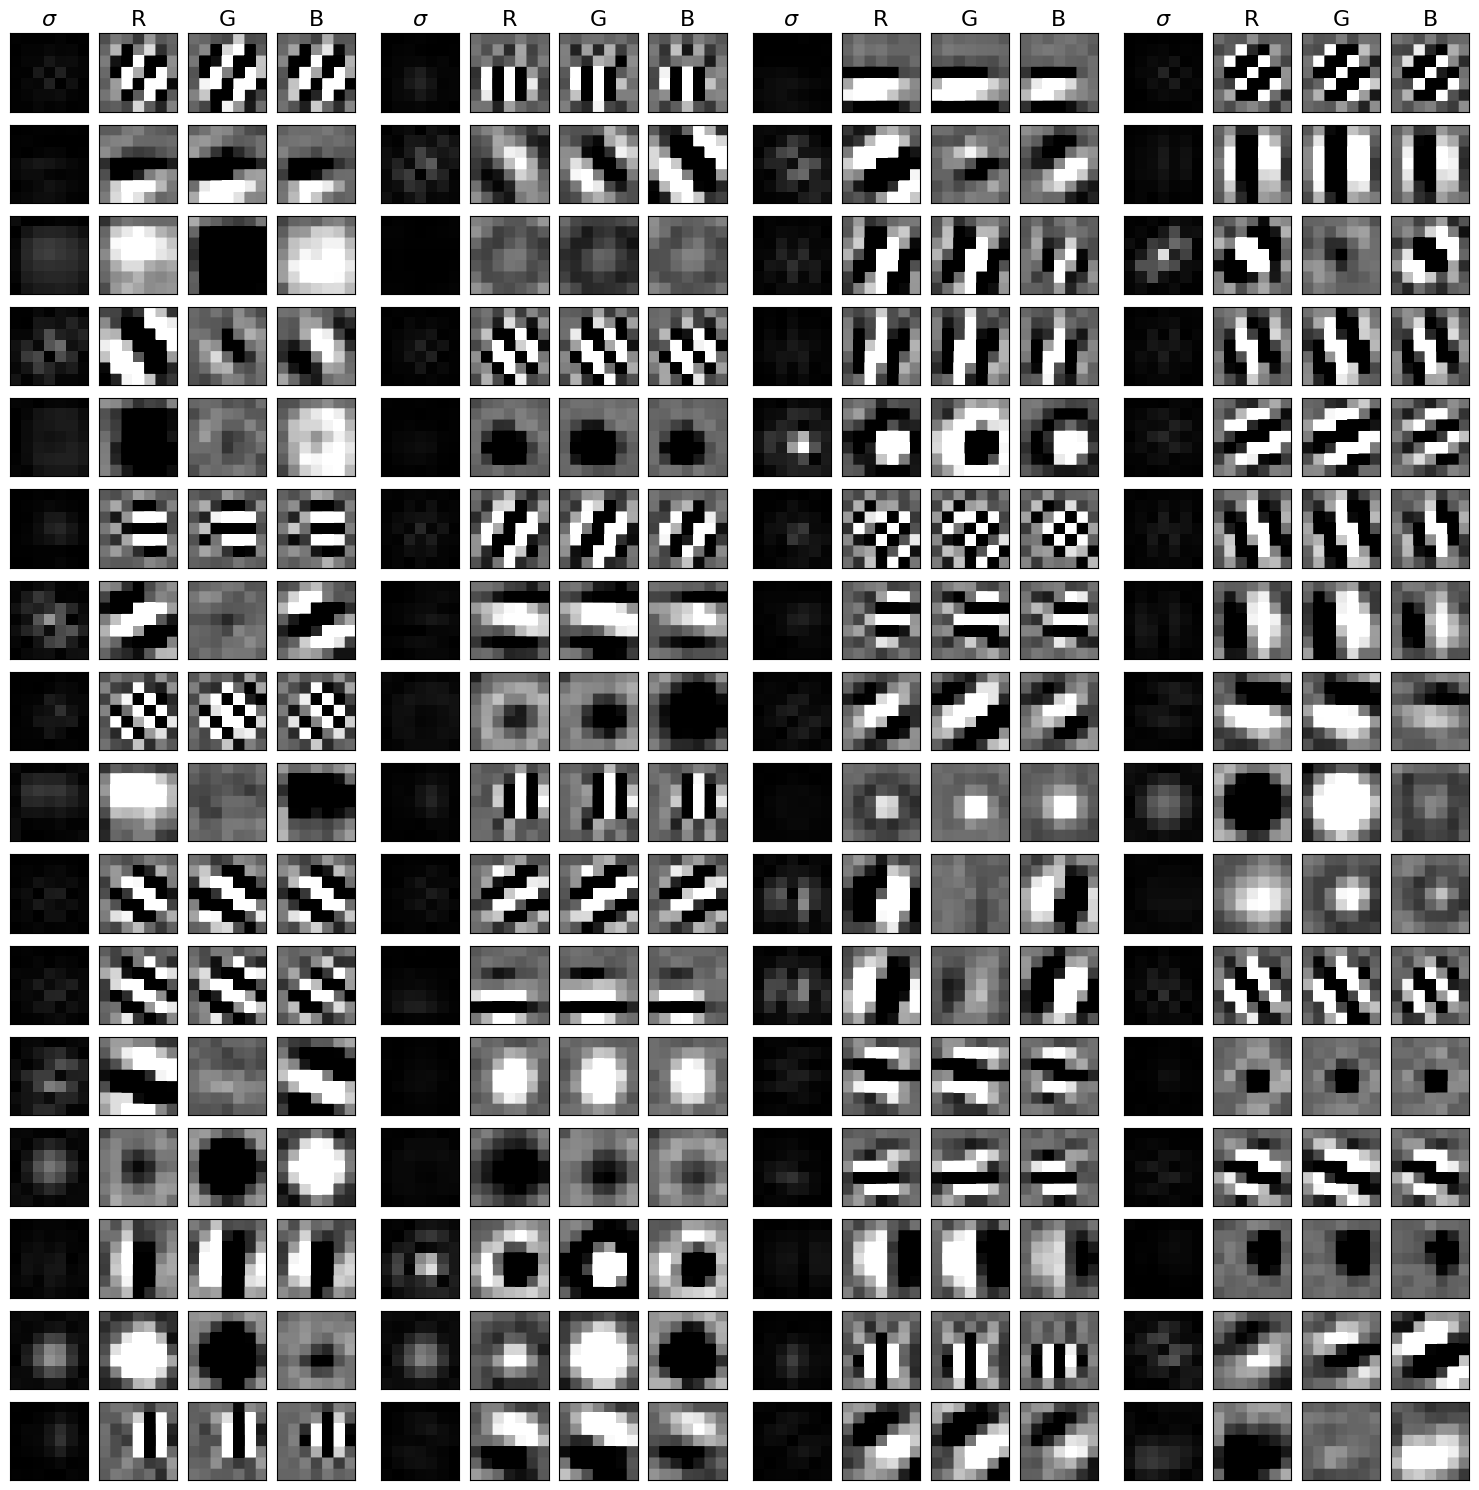}
          \caption{\scriptsize{resnext\_101}}\label{magface_meanshift}
      \end{subfigure}
      \hfill
      \begin{subfigure}[b]{0.3\linewidth}
        \centering
          \includegraphics[width=1\linewidth]{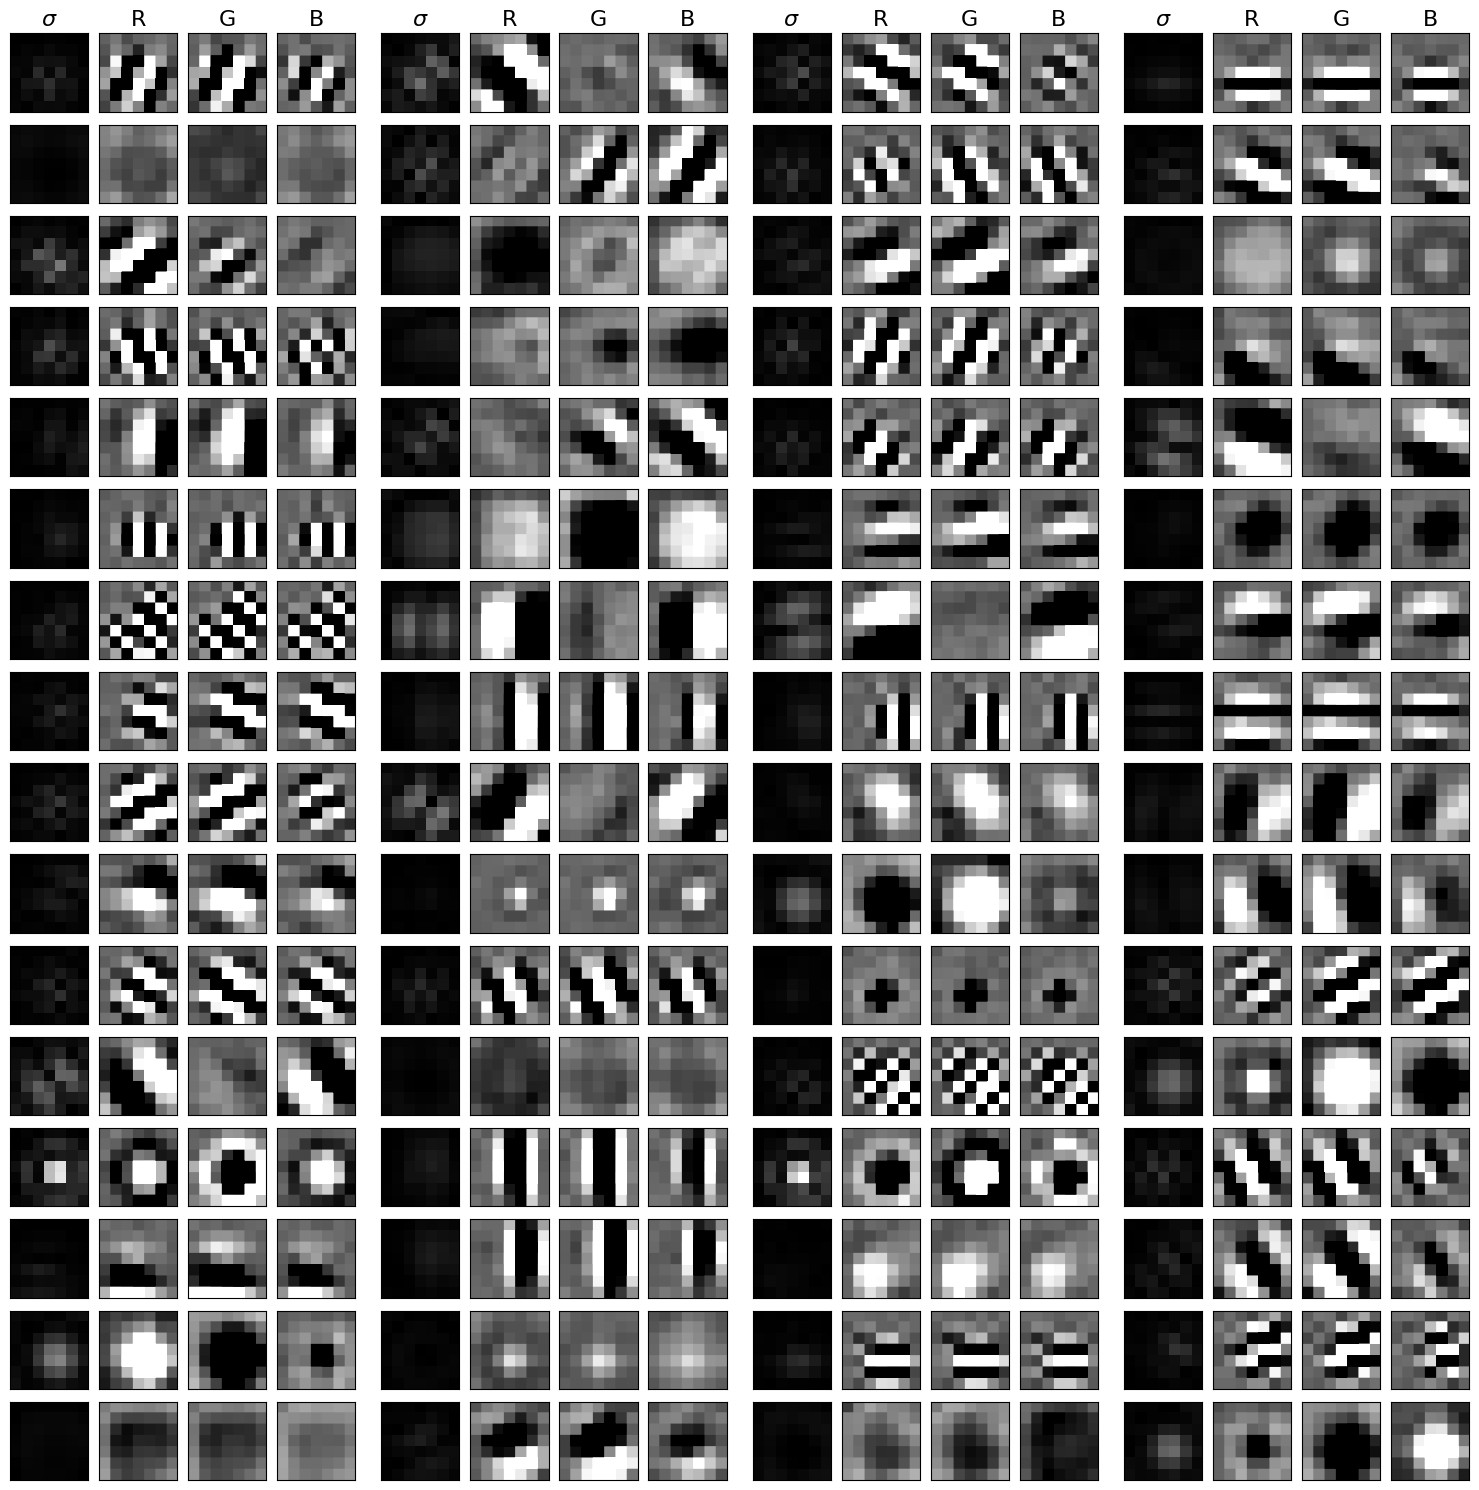}
          \caption{\scriptsize{wideresnet\_101}}\label{magface_meanshift}
      \end{subfigure}
  \end{subfigure}
  \caption{General Classification Models}\label{classification}
  \label{fig:general classification}
  \vspace{-1em}
\end{figure*}
