# Supplementary material for: CRAFT: Contextual Re-Activation of Filters for face recognition Training
Source: arXiv:2312.00072 source file (2023-12-05)
Supplement: Supplementary file 2 [file baseline_vs_complementary.tex]

\begin{figure*}[ht!]
 \centering
  \begin{subfigure}[b]{.6\linewidth}
      \begin{subfigure}[b]{0.475\linewidth}
        \centering
          \includegraphics[width=1\linewidth]{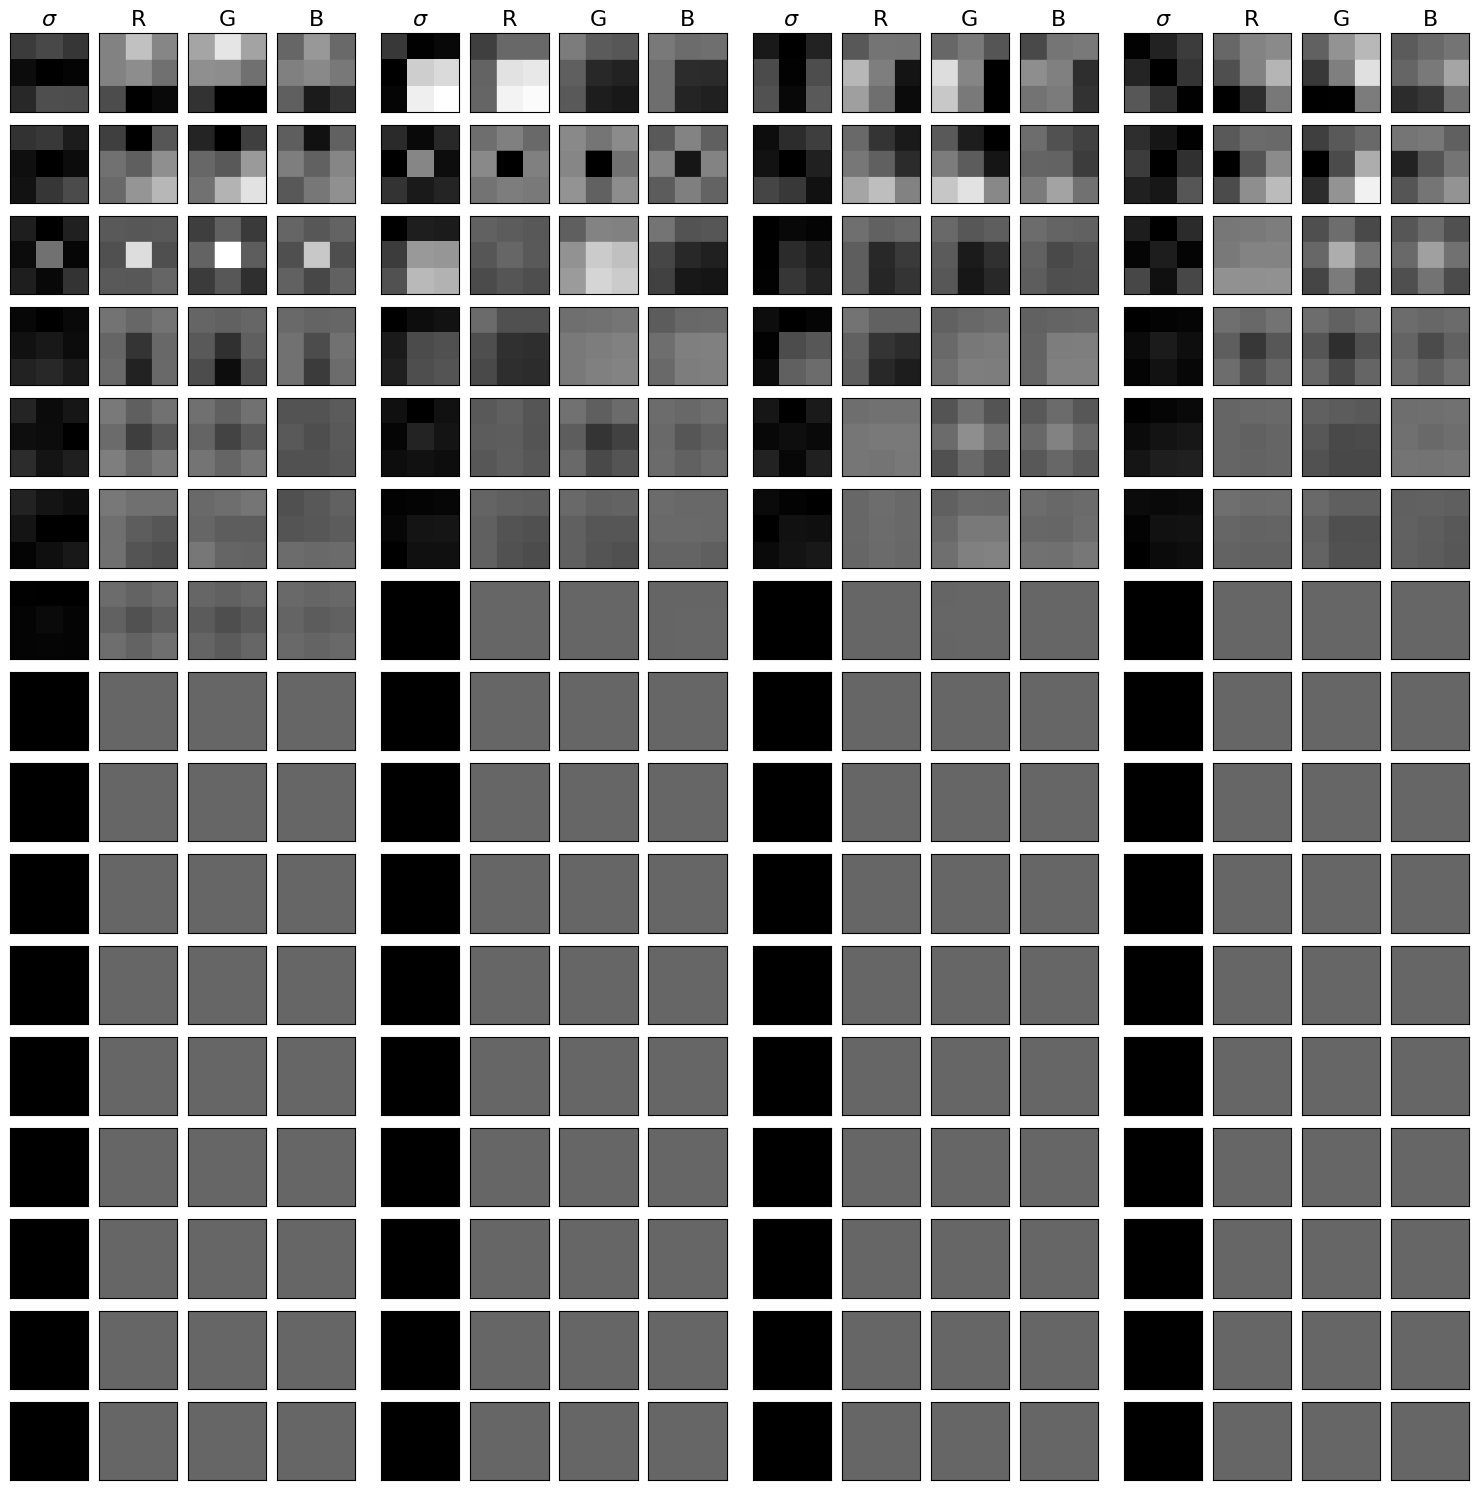}
          \caption{\scriptsize{Baseline Method (No-Reactivation)}}\label{noreint}
      \end{subfigure}
      \hfill
      \begin{subfigure}[b]{0.475\linewidth}
        \centering
          \includegraphics[width=1\linewidth]{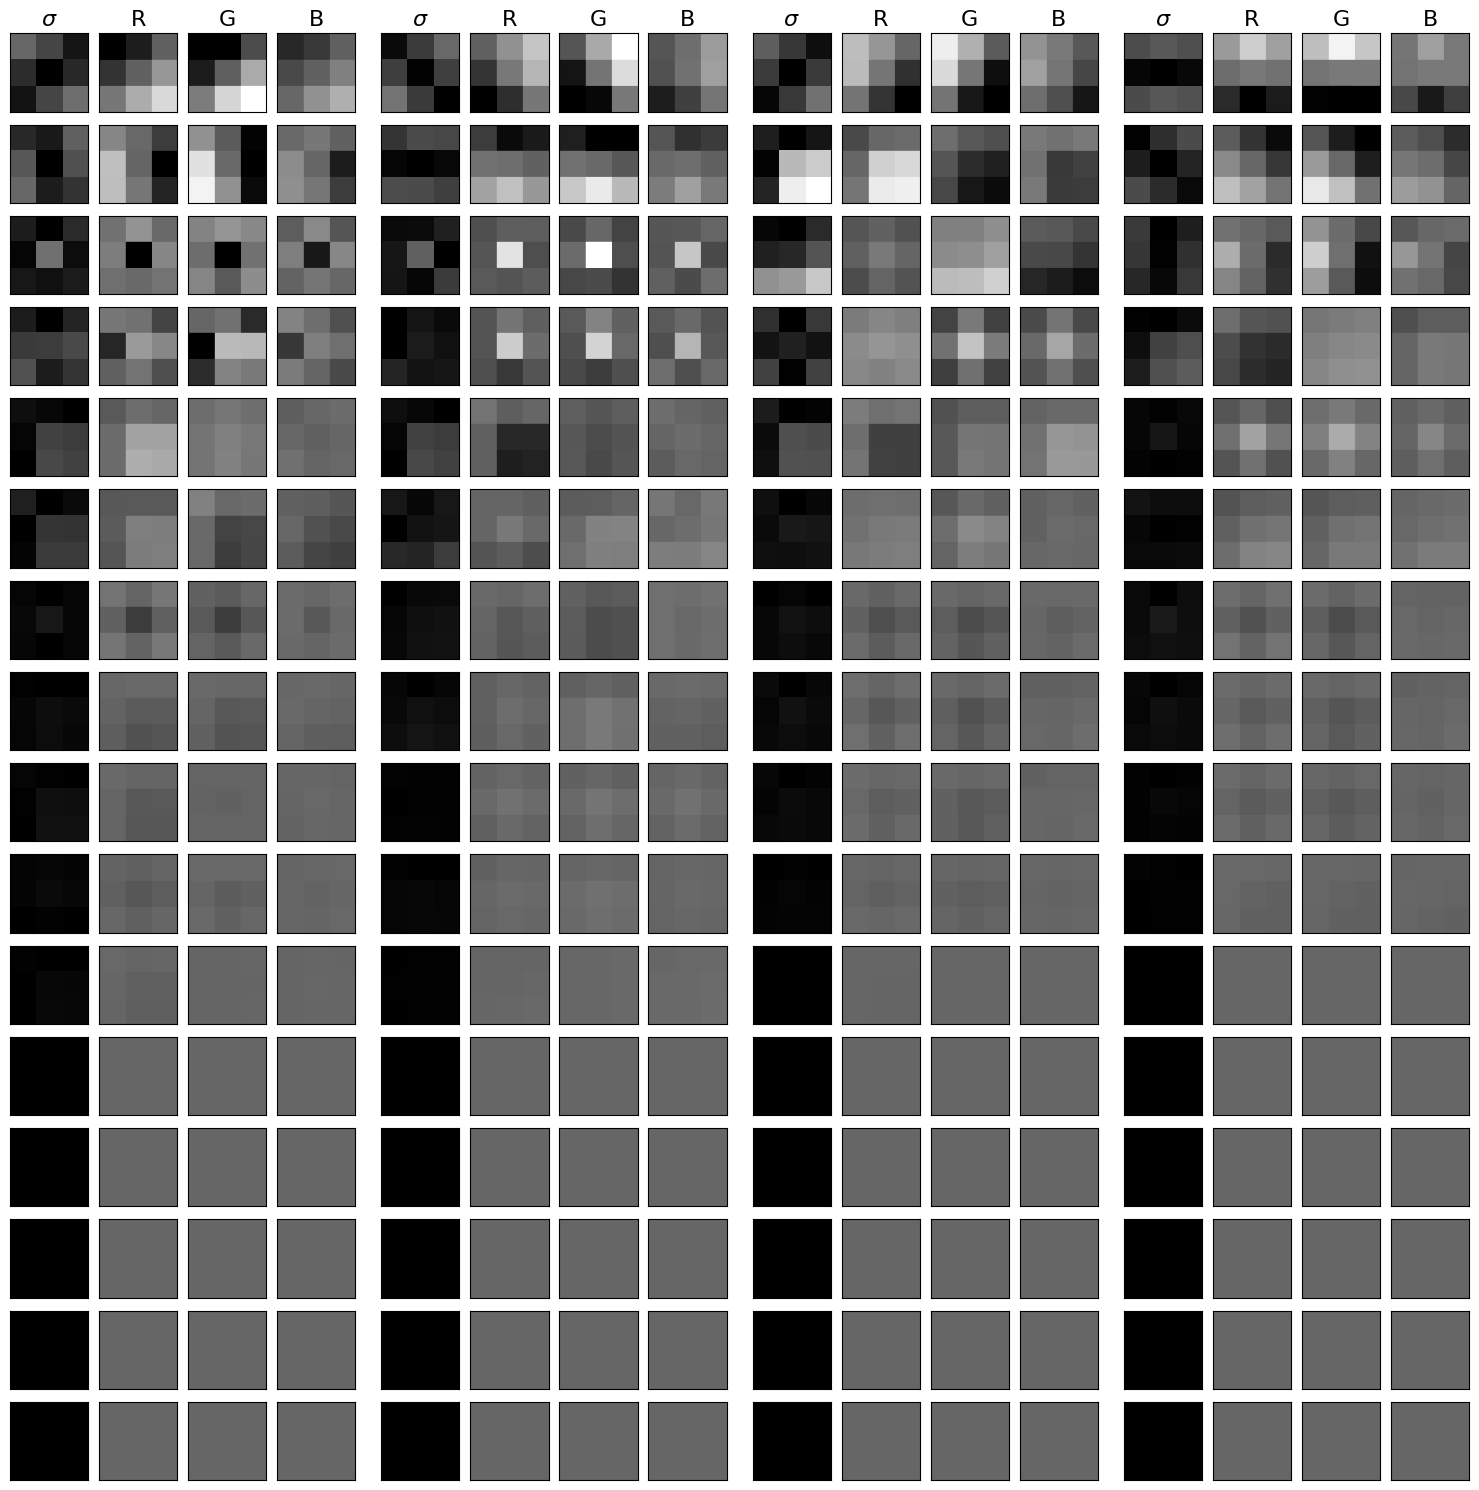}
          \caption{\scriptsize{ Directed Complementary Reactivation}}\label{highflipped}
      \end{subfigure}
  \end{subfigure}
  \caption{\textbf{Visualization of 64 Convolution Filter Weight Values for the First Convolution Block in row-major order.} Filters are presented in the row-major order based on the L1-norm ranking from top left grid position to the bottom right. The figure illustrates that the model trained using the standard training setup (without reactivation) has more ``inactive" filters in comparison to the model trained with CRAFT.}
  \label{fig:weight_vis}
\end{figure*}
