# Supplementary material for: CRAFT: Contextual Re-Activation of Filters for face recognition Training
Source: arXiv:2312.00072 source file (2023-12-05)
Supplement: Supplementary file 3 [file instance_segmentation.tex]

\begin{figure*}[ht!]
 \centering
  \begin{subfigure}[b]{0.9\linewidth}
  \centering
      \begin{subfigure}[b]{0.5\linewidth}
        \centering
          \includegraphics[width=1\linewidth]{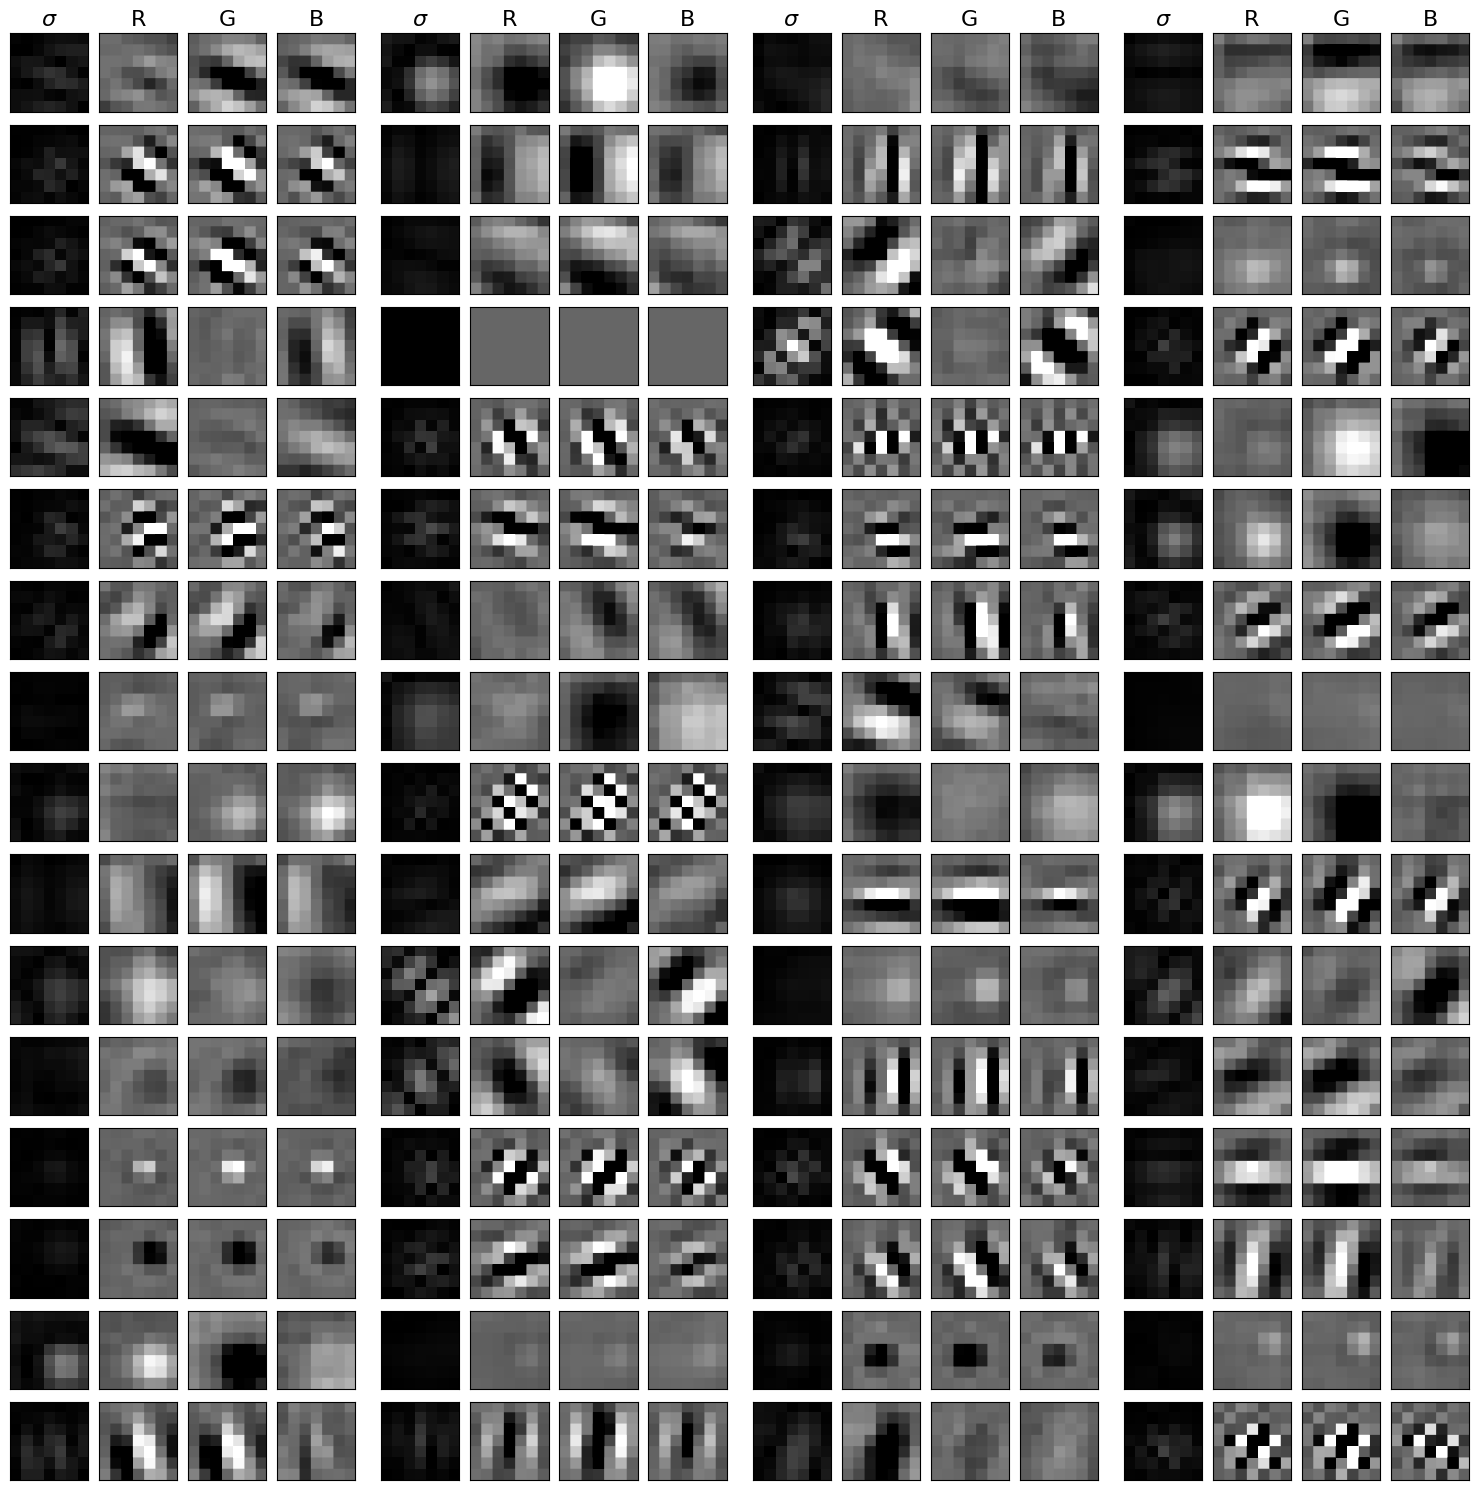}
          \caption{\scriptsize{mask-rcnn-r50}}\label{maskrcnn}
      \end{subfigure}
  \end{subfigure}
  \caption{Instance Segmenatation Model}
  \label{fig:instance_segmentation_models}
  \vspace{-1em}
\end{figure*}
