# Supplementary material for: CRAFT: Contextual Re-Activation of Filters for face recognition Training
Source: arXiv:2312.00072 source file (2023-12-05)
Supplement: Supplementary file 4 [file semantic_segmentation.tex]

\begin{figure*}[ht!]
 \centering
  \begin{subfigure}[b]{0.9\linewidth}
      \begin{subfigure}[b]{0.3\linewidth}
        \centering
          \includegraphics[width=1\linewidth]{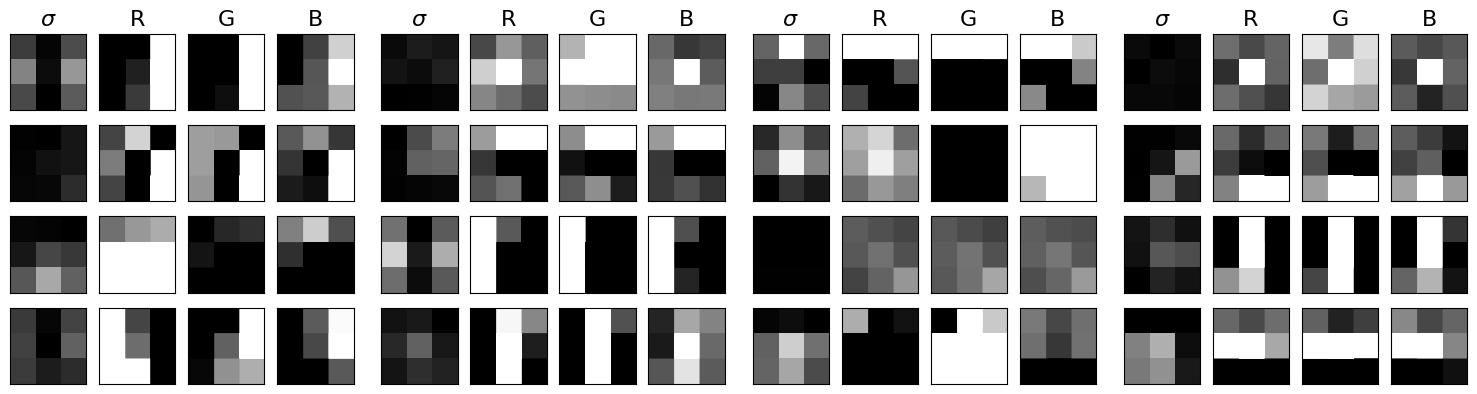}
          \caption{\scriptsize{lraspp-mobilenet-v3-large}}\label{lraspp}
      \end{subfigure}
      \hfill
      \begin{subfigure}[b]{0.3\linewidth}
        \centering
          \includegraphics[width=1\linewidth]{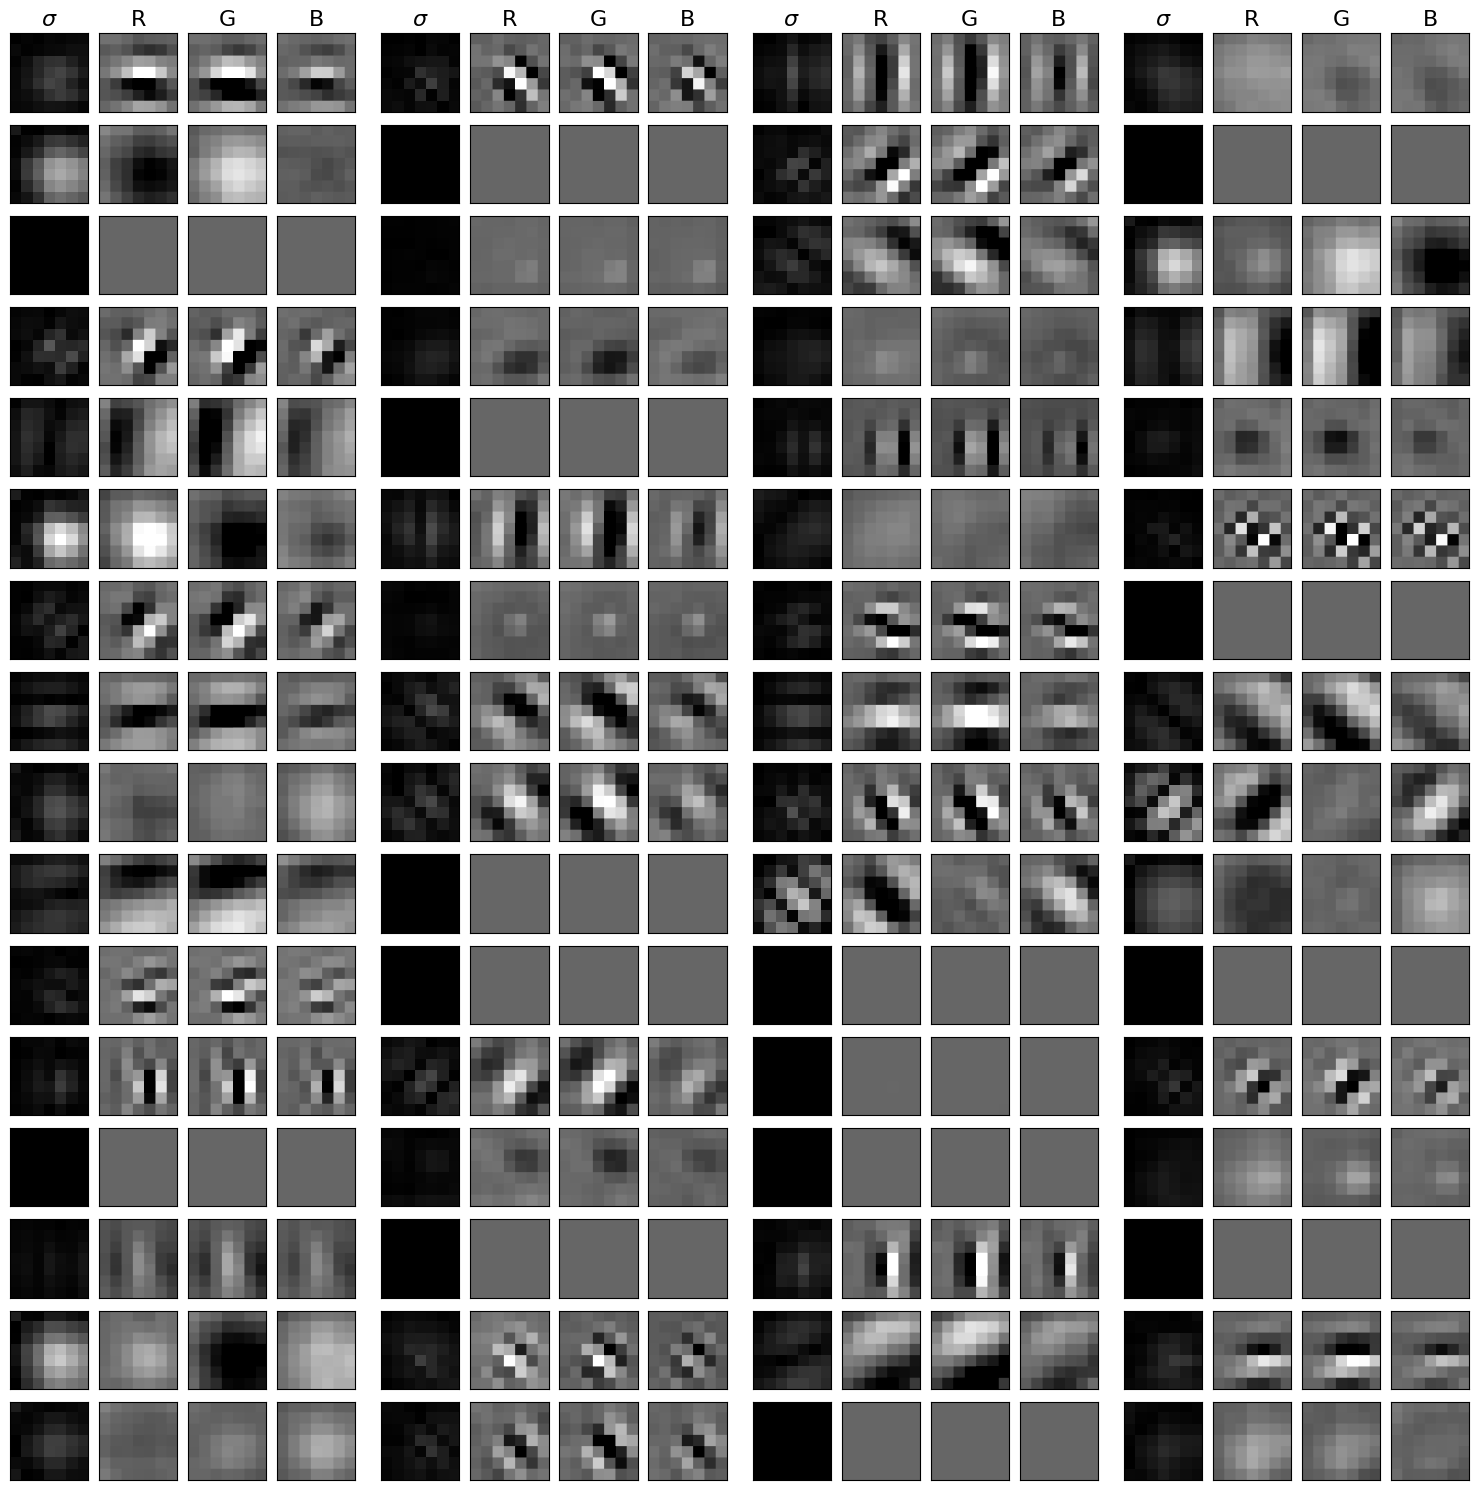}
          \caption{\scriptsize{fcn-resnet101}}\label{fcn}
      \end{subfigure}
      \hfill
      \begin{subfigure}[b]{0.3\linewidth}
        \centering
          \includegraphics[width=1\linewidth]{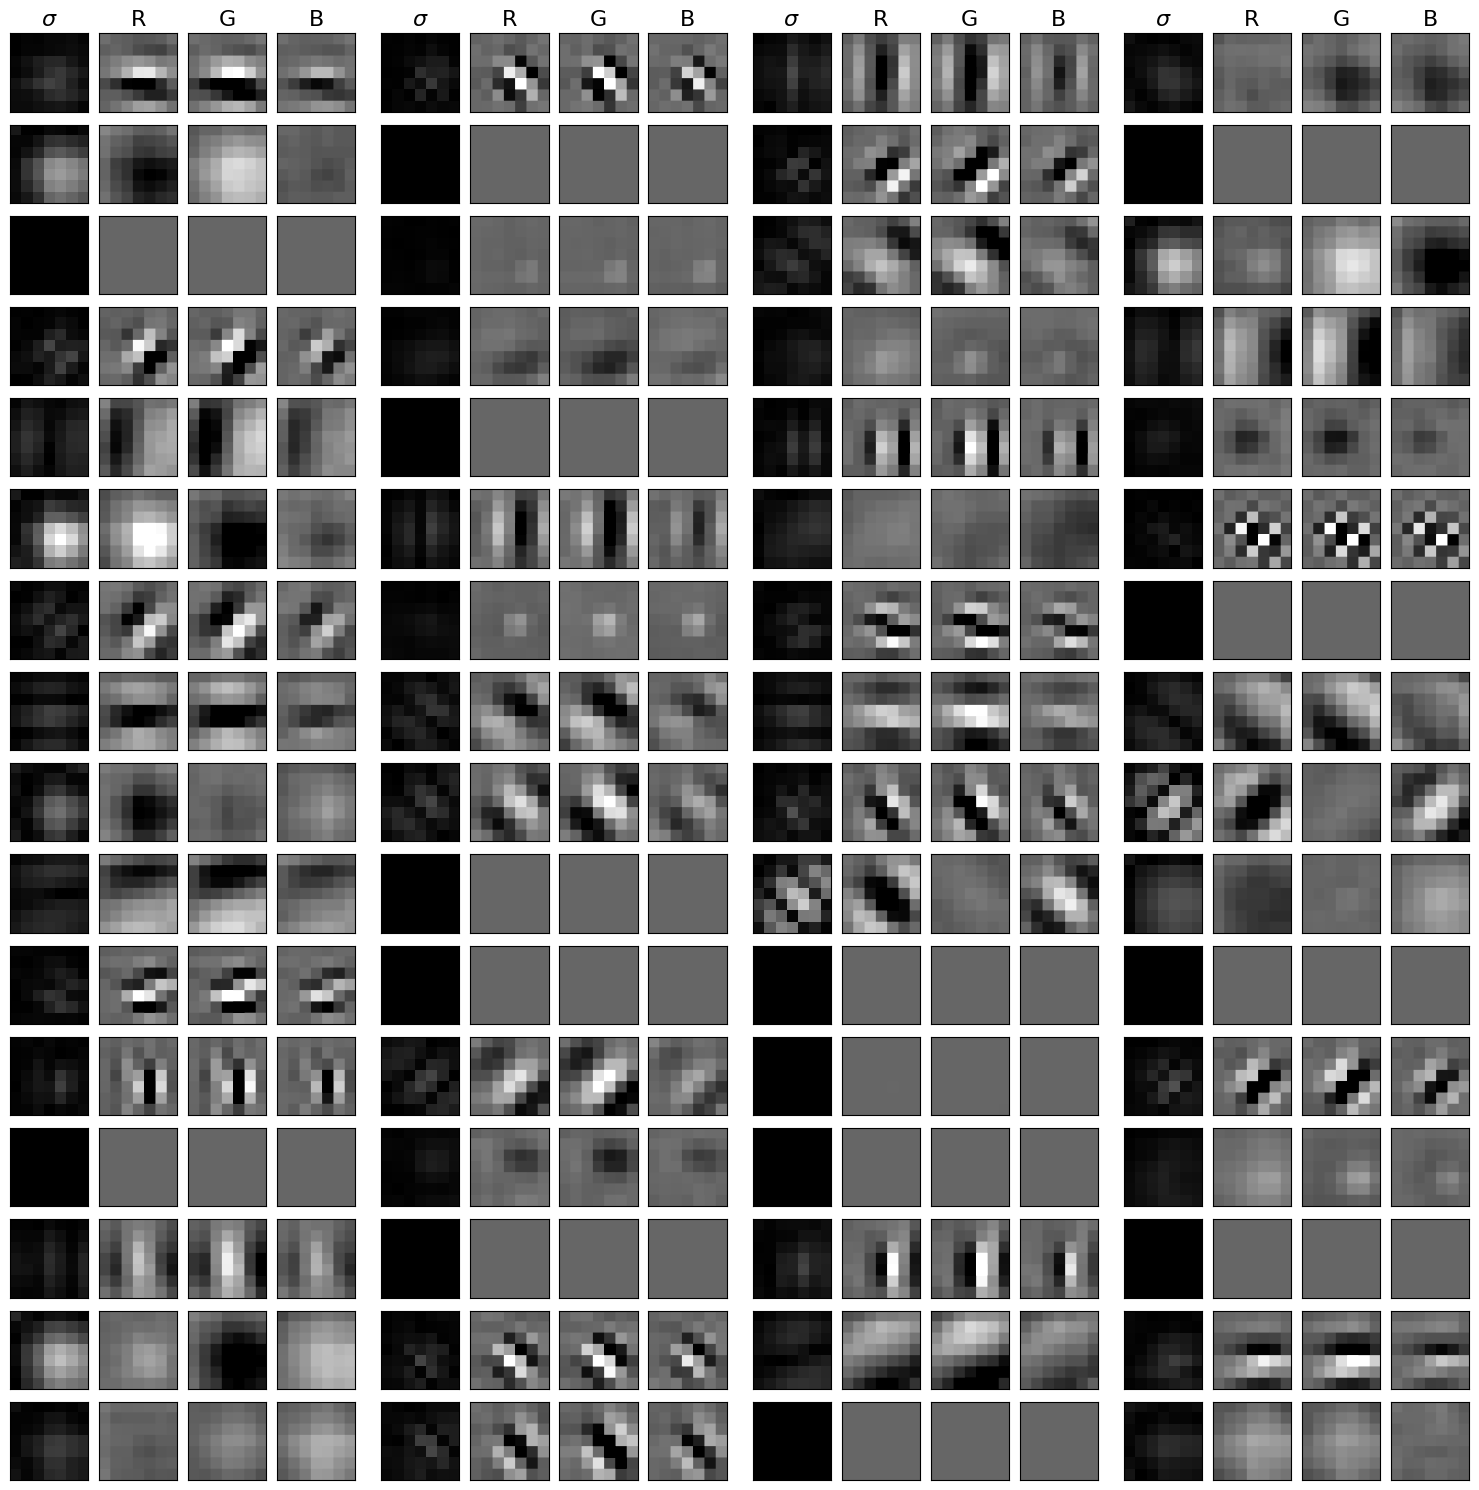}
          \caption{\scriptsize{deeplabv3-resnet101}}\label{deeplabv3}
      \end{subfigure}
  \end{subfigure}
  \caption{Semantic Segmentation Models}
  \label{fig:semantic_segmentation_model}
  \vspace{-1em}
\end{figure*}
