# Supplementary material for: CRAFT: Contextual Re-Activation of Filters for face recognition Training
Source: arXiv:2312.00072 source file (2023-12-05)
Supplement: Supplementary file 5 [file table.tex]

\begin{table}[!ht]
\raggedright
\resizebox{.3\columnwidth}{!}{
\begin{tabular}{|c|c|}
\hline
Pre-trained-Models  & Number of ``inactive" filters \\\hline
magface-r100-ms1mv2 & 41                            \\\hline
magface-r50-ms1mv2  & 34                            \\\hline
adaface-r100-ms1mv2 & 13                            \\\hline
adaface-r100-ms1mv2 & 13                           \\\hline
\end{tabular}
}
\vspace{0.2cm}

    {\scriptsize Total Number of Filters ($N$) = 64 \\
    $\theta$ (threshold used to identify ``inactive" filters) = $1e^{-3}$} 
\caption{``inactive" filters in other popular face-recognition models. }
\label{tab:my-table}
\end{table}
