# Supplementary material for: CRAFT: Contextual Re-Activation of Filters for face recognition Training
Source: arXiv:2312.00072 source file (2023-12-05)
Supplement: Supplementary file 6 [file weight_transform.tex]

\centering
\begin{figure*}[ht!]
 \centering
 \includegraphics[width=\linewidth]{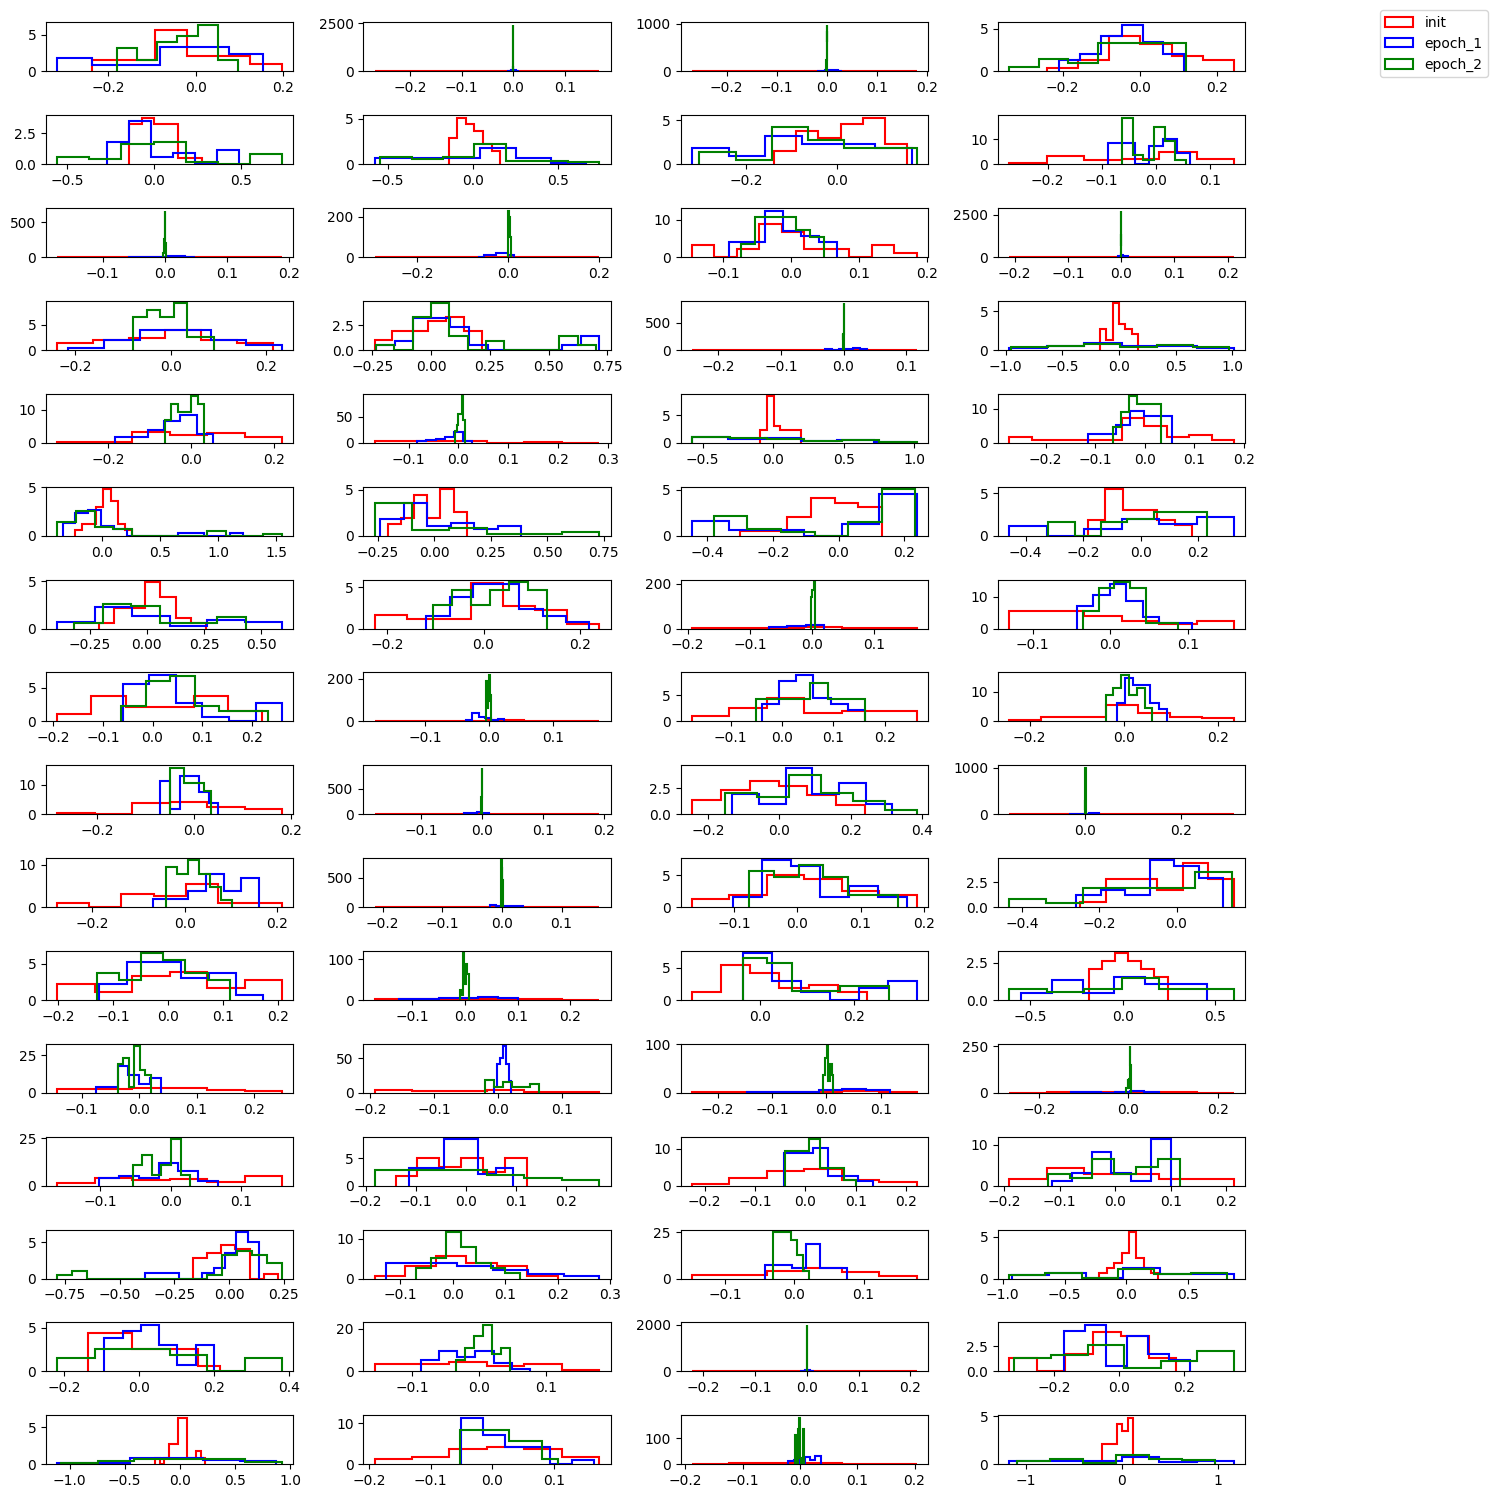}
  \caption{During training, the filter weights' distribution quickly shifts away from being Gaussian}\label{weight_track}
  \label{fig:weight-transform}
  \vspace{-1em}
\end{figure*}
